# Supplementary material for: Concept-Based Mechanistic Interpretability Using Structured Knowledge Graphs
Source: arXiv:2507.05810 source file (2025-07-08)
Supplement: Supplementary file 1 [file appendix_1.tex]

\appendix
\label{appndx:results}

The values in the tables correspond to the probability of a concept being detected in the feature map produced by the model at a particular layer (the probability is average (Avg) over all concepts). We identify the threshold that yields the maximum probability and provide its value in parentheses. The rows are sorted in descending order of model's accuracy (Acc $\uparrow$). Cells representing the highest probability for each model are marked in bold, while those with the second-best probability are indicated in blue.

\begin{table}[h]
\centering

\caption{KitFoxVsRedFox. Weighted F1-scores}
\begin{tabular}{|l|c|c|c|c|c|c|c|}
\hline
Model & Layer 1 & Layer 2 & Layer 3 & Layer 4 & Layer 5 & Avg. F1  $\uparrow$ & Acc. $\uparrow$ \\ \hline
ResNeXt101 & 0.794 & 0.843 & 0.867 & \color{blue}{0.906} & \textbf{0.922} & 0.866 & 0.760 \\
AlexNet & 0.765 & \color{blue}{0.865} & \color{blue}{0.865} & \textbf{0.890} & 0.863 & 0.850 & 0.700 \\
ResNeXt50 & 0.777 & \color{blue}{0.897} & 0.872 & 0.858 & \textbf{0.903} & 0.861 & 0.700 \\
DenseNet121 & 0.714 & 0.886 & 0.863 & \color{blue}{0.897} & \textbf{0.904} & 0.853 & 0.700 \\
VGG16 & 0.818 & 0.797 & \textbf{0.883} & \color{blue}{0.865} & 0.842 & 0.841 & 0.700 \\
DenseNet169 & 0.773 & 0.863 & 0.848 & \color{blue}{0.908} & \textbf{0.922} & 0.863 & 0.690 \\
Googlelenet & 0.860 & 0.810 & 0.845 & \color{blue}{0.869} & \textbf{0.896} & 0.856 & 0.670 \\
EfficientNet & 0.835 & 0.770 & 0.832 & \color{blue}{0.870} & \textbf{0.871} & 0.836 & 0.630 \\
Resnet18 & 0.762 & 0.823 & 0.849 & \color{blue}{0.867} & \textbf{0.868} & 0.834 & 0.610 \\
\hline
\end{tabular}
\label{tab:kitfoxvsredfox_bias_f1}
\end{table}

\begin{table}[h]
\centering

\caption{KitFoxVsRedFox. JS divergence}
\begin{tabular}{|l|c|c|c|c|c|c|c|}
\hline
Model & Layer 1 & Layer 2 & Layer 3 & Layer 4 & Layer 5 & Avg. JS  $\downarrow$ & Acc. $\uparrow$ \\ \hline
ResNeXt101 & 0.111 & 0.090 & 0.073 & \color{blue}{0.054} & \textbf{0.047} & 0.075 & 0.760 \\
AlexNet & 0.133 & 0.064 & 0.055 & \color{blue}{0.052} & \textbf{0.051} & 0.071 & 0.700 \\
ResNeXt50 & 0.112 & \color{blue}{0.051} & 0.071 & 0.057 & \textbf{0.049} & 0.068 & 0.700 \\
DenseNet121 & 0.135 & \color{blue}{0.060} & 0.077 & 0.063 & \textbf{0.059} & 0.079 & 0.700 \\
VGG16 & 0.120 & 0.070 & \color{blue}{0.056} & \textbf{0.050} & 0.075 & 0.074 & 0.700 \\
DenseNet169 & 0.123 & 0.063 & 0.078 & \color{blue}{0.059} & \textbf{0.054} & 0.075 & 0.690 \\
Googlelenet & 0.081 & 0.091 & 0.073 & \textbf{0.058} & \color{blue}{0.059} & 0.072 & 0.670 \\
EfficientNet & 0.098 & 0.109 & \color{blue}{0.089} & 0.092 & \textbf{0.056} & 0.089 & 0.630 \\
Resnet18 & 0.119 & 0.079 & 0.091 & \color{blue}{0.075} & \textbf{0.066} & 0.086 & 0.610 \\
\hline
\end{tabular}
\label{tab:kitfoxvsredfox_bias_js}
\end{table}

Correlations with Accuracy: F1 (0.783), JS Divergence (-0.690)

\newpage

\begin{table}[h]
\centering

\caption{HuskyVsWolf. Weighted F1-scores}
\begin{tabular}{|l|c|c|c|c|c|c|c|}
\hline
Model & Layer 1 & Layer 2 & Layer 3 & Layer 4 & Layer 5 & Avg. F1  $\uparrow$ & Acc. $\uparrow$ \\ \hline
DenseNet121 & 0.598 & 0.851 & 0.838 & \color{blue}{0.852} & \textbf{0.904} & 0.808 & 0.980 \\
ResNeXt101 & 0.733 & 0.869 & \textbf{0.908} & \color{blue}{0.878} & \textbf{0.908} & 0.859 & 0.980 \\
VGG16 & 0.686 & 0.793 & \color{blue}{0.863} & 0.821 & \textbf{0.868} & 0.806 & 0.970 \\
EfficientNet & 0.724 & 0.774 & \color{blue}{0.857} & 0.818 & \textbf{0.907} & 0.816 & 0.960 \\
Googlelenet & 0.775 & 0.836 & \color{blue}{0.889} & \textbf{0.894} & 0.867 & 0.852 & 0.960 \\
ResNeXt50 & 0.582 & 0.809 & 0.850 & \color{blue}{0.892} & \textbf{0.932} & 0.813 & 0.960 \\
DenseNet169 & 0.558 & 0.826 & 0.842 & \color{blue}{0.889} & \textbf{0.903} & 0.804 & 0.960 \\
Resnet18 & 0.556 & \textbf{0.884} & 0.812 & 0.868 & \color{blue}{0.870} & 0.798 & 0.950 \\
AlexNet & 0.685 & 0.828 & 0.832 & \textbf{0.894} & \color{blue}{0.889} & 0.826 & 0.940 \\
\hline
\end{tabular}
\label{tab:huskyvswolf_bias_f1}
\end{table}

\begin{table}[h]
\centering

\caption{HuskyVsWolf. JS divergence}
\begin{tabular}{|l|c|c|c|c|c|c|c|}
\hline
Model & Layer 1 & Layer 2 & Layer 3 & Layer 4 & Layer 5 & Avg. JS  $\downarrow$ & Acc. $\uparrow$ \\ \hline
DenseNet121 & 0.168 & \color{blue}{0.069} & 0.082 & \color{blue}{0.069} & \textbf{0.064} & 0.091 & 0.980 \\
ResNeXt101 & 0.155 & 0.100 & 0.078 & \color{blue}{0.062} & \textbf{0.057} & 0.090 & 0.980 \\
VGG16 & 0.162 & 0.088 & \color{blue}{0.069} & \textbf{0.059} & 0.078 & 0.091 & 0.970 \\
EfficientNet & 0.129 & 0.141 & \color{blue}{0.095} & 0.098 & \textbf{0.061} & 0.105 & 0.960 \\
Googlelenet & 0.118 & 0.097 & 0.074 & \textbf{0.062} & \color{blue}{0.066} & 0.083 & 0.960 \\
ResNeXt50 & 0.170 & 0.103 & 0.078 & \color{blue}{0.061} & \textbf{0.057} & 0.094 & 0.960 \\
DenseNet169 & 0.169 & 0.070 & 0.082 & \color{blue}{0.064} & \textbf{0.060} & 0.089 & 0.960 \\
Resnet18 & 0.171 & 0.095 & 0.101 & \color{blue}{0.079} & \textbf{0.072} & 0.103 & 0.950 \\
AlexNet & 0.164 & 0.085 & 0.063 & \textbf{0.057} & \color{blue}{0.058} & 0.085 & 0.940 \\
\hline
\end{tabular}
\label{tab:huskyvswolf_bias_js}
\end{table}

Correlations with accuracy: F1 (0.229), JS Divergence (-0.078)

\newpage

\begin{table}[h]
\centering

\caption{manumoi. Weighted F1-scores}
\begin{tabular}{|l|c|c|c|c|c|c|c|}
\hline
Model & Layer 1 & Layer 2 & Layer 3 & Layer 4 & Layer 5 & Avg. F1  $\uparrow$ & Acc. $\uparrow$ \\ \hline
EfficientNet & 0.833 & 0.654 & 0.804 & \textbf{0.881} & \textbf{0.881} & 0.811 & 0.914 \\
DenseNet169 & 0.767 & 0.950 & \textbf{1.000} & 0.917 & \textbf{1.000} & 0.927 & 0.901 \\
Googlelenet & 0.833 & \textbf{0.867} & \textbf{0.867} & 0.831 & \textbf{0.867} & 0.853 & 0.901 \\
DenseNet121 & 0.767 & 0.867 & \color{blue}{0.917} & \textbf{1.000} & 0.833 & 0.877 & 0.888 \\
ResNeXt50 & 0.767 & \textbf{0.867} & \textbf{0.867} & 0.831 & \textbf{0.867} & 0.840 & 0.868 \\
Resnet18 & 0.750 & 0.798 & \color{blue}{0.831} & \textbf{0.917} & 0.798 & 0.819 & 0.865 \\
VGG16 & 0.446 & 0.798 & \color{blue}{0.867} & \textbf{0.917} & \color{blue}{0.867} & 0.779 & 0.851 \\
AlexNet & 0.731 & 0.867 & \textbf{1.000} & \color{blue}{0.964} & \color{blue}{0.964} & 0.905 & 0.848 \\
ResNeXt101 & 0.767 & \color{blue}{0.917} & \textbf{0.950} & 0.833 & 0.833 & 0.860 & 0.812 \\
\hline
\end{tabular}
\label{tab:manumoi_bias_f1}
\end{table}

\begin{table}[h]
\centering

\caption{manumoi. JS divergence}
\begin{tabular}{|l|c|c|c|c|c|c|c|}
\hline
Model & Layer 1 & Layer 2 & Layer 3 & Layer 4 & Layer 5 & Avg. JS  $\downarrow$ & Acc. $\uparrow$ \\ \hline
EfficientNet & 0.366 & 0.358 & 0.278 & \textbf{0.164} & \color{blue}{0.228} & 0.279 & 0.914 \\
DenseNet169 & 0.418 & 0.137 & 0.150 & \color{blue}{0.123} & \textbf{0.119} & 0.189 & 0.901 \\
Googlelenet & 0.291 & 0.181 & \color{blue}{0.132} & 0.228 & \textbf{0.115} & 0.189 & 0.901 \\
DenseNet121 & 0.417 & \color{blue}{0.134} & 0.145 & \textbf{0.123} & 0.228 & 0.209 & 0.888 \\
ResNeXt50 & 0.416 & \color{blue}{0.192} & \textbf{0.137} & 0.240 & 0.237 & 0.244 & 0.868 \\
Resnet18 & 0.425 & 0.259 & \color{blue}{0.191} & \textbf{0.138} & 0.232 & 0.249 & 0.865 \\
VGG16 & 0.428 & 0.253 & 0.157 & \textbf{0.100} & \color{blue}{0.132} & 0.214 & 0.851 \\
AlexNet & 0.411 & 0.255 & 0.133 & \color{blue}{0.122} & \textbf{0.106} & 0.206 & 0.848 \\
ResNeXt101 & 0.416 & \textbf{0.131} & \color{blue}{0.135} & 0.233 & 0.249 & 0.233 & 0.812 \\
\hline
\end{tabular}
\label{tab:manumoi_bias_js}
\end{table}

Correlations with Accuracy: F1 (0.073), JS Divergence (-0.011)

\newpage

\begin{table}[h]
\centering

\caption{derm7pt. Weighted F1-scores}
\begin{tabular}{|l|c|c|c|c|c|c|c|}
\hline
Model & Layer 1 & Layer 2 & Layer 3 & Layer 4 & Layer 5 & Avg. F1  $\uparrow$ & Acc. $\uparrow$ \\ \hline
Resnet18 & 0.343 & 0.496 & 0.514 & \color{blue}{0.570} & \textbf{0.584} & 0.501 & 0.513 \\
Googlelenet & 0.501 & 0.515 & \color{blue}{0.607} & \textbf{0.616} & 0.395 & 0.527 & 0.492 \\
DenseNet169 & 0.337 & \textbf{0.576} & 0.506 & \textbf{0.576} & 0.573 & 0.514 & 0.492 \\
AlexNet & 0.449 & 0.476 & \color{blue}{0.570} & 0.532 & \textbf{0.619} & 0.529 & 0.492 \\
VGG16 & 0.368 & 0.509 & \color{blue}{0.529} & \textbf{0.620} & 0.521 & 0.509 & 0.477 \\
EfficientNet & 0.405 & 0.415 & \textbf{0.532} & \color{blue}{0.524} & 0.505 & 0.476 & 0.472 \\
ResNeXt50 & 0.321 & \color{blue}{0.541} & 0.535 & \textbf{0.581} & 0.531 & 0.502 & 0.447 \\
DenseNet121 & 0.317 & \textbf{0.604} & \color{blue}{0.576} & 0.556 & 0.562 & 0.523 & 0.442 \\
ResNeXt101 & 0.360 & 0.475 & \textbf{0.557} & \color{blue}{0.526} & 0.446 & 0.473 & 0.397 \\
\hline
\end{tabular}
\label{tab:derm7pt_bias_f1}
\end{table}

\begin{table}[h]
\centering

\caption{derm7pt. JS divergence}
\begin{tabular}{|l|c|c|c|c|c|c|c|}
\hline
Model & Layer 1 & Layer 2 & Layer 3 & Layer 4 & Layer 5 & Avg. JS  $\downarrow$ & Acc. $\uparrow$ \\ \hline
Resnet18 & 0.484 & 0.426 & 0.445 & \color{blue}{0.424} & \textbf{0.423} & 0.440 & 0.513 \\
Googlelenet & 0.438 & 0.446 & \color{blue}{0.429} & \textbf{0.422} & 0.444 & 0.436 & 0.492 \\
DenseNet169 & 0.461 & \textbf{0.406} & 0.435 & \color{blue}{0.414} & 0.423 & 0.428 & 0.492 \\
AlexNet & 0.442 & 0.432 & \color{blue}{0.386} & 0.395 & \textbf{0.379} & 0.407 & 0.492 \\
VGG16 & 0.483 & 0.429 & \color{blue}{0.387} & \textbf{0.382} & 0.434 & 0.423 & 0.477 \\
EfficientNet & 0.480 & 0.456 & \textbf{0.432} & 0.448 & \textbf{0.432} & 0.450 & 0.472 \\
ResNeXt50 & 0.483 & 0.444 & \color{blue}{0.425} & \textbf{0.423} & 0.426 & 0.440 & 0.447 \\
DenseNet121 & 0.483 & \textbf{0.401} & 0.425 & \color{blue}{0.412} & 0.420 & 0.428 & 0.442 \\
ResNeXt101 & 0.461 & 0.448 & \color{blue}{0.425} & \textbf{0.413} & 0.439 & 0.437 & 0.397 \\
\hline
\end{tabular}
\label{tab:derm7pt_bias_js}
\end{table}

Correlations with Accuracy: F1 (0.514), JS Divergence (-0.199)

\newpage

\begin{table}[h]
\centering

\caption{CatsDogsBiased. Weighted F1-scores}
\begin{tabular}{|l|c|c|c|c|c|c|c|}
\hline
Model & Layer 1 & Layer 2 & Layer 3 & Layer 4 & Layer 5 & Avg. F1  $\uparrow$ & Acc. $\uparrow$ \\ \hline
ResNeXt101 & 0.805 & 0.841 & \textbf{0.862} & \color{blue}{0.844} & 0.815 & 0.834 & 0.914 \\
ResNeXt50 & 0.801 & 0.845 & \textbf{0.862} & 0.846 & \color{blue}{0.859} & 0.842 & 0.876 \\
VGG16 & 0.797 & \textbf{0.872} & \color{blue}{0.855} & 0.825 & 0.809 & 0.832 & 0.784 \\
DenseNet169 & 0.797 & \textbf{0.880} & \color{blue}{0.870} & 0.848 & 0.834 & 0.846 & 0.782 \\
DenseNet121 & 0.797 & \color{blue}{0.861} & \textbf{0.881} & 0.852 & 0.826 & 0.843 & 0.761 \\
Resnet18 & 0.794 & \textbf{0.863} & 0.820 & \color{blue}{0.846} & 0.810 & 0.827 & 0.679 \\
Googlelenet & \color{blue}{0.855} & 0.837 & \textbf{0.883} & 0.843 & 0.810 & 0.845 & 0.643 \\
EfficientNet & 0.818 & 0.797 & \color{blue}{0.840} & 0.809 & \textbf{0.867} & 0.826 & 0.586 \\
AlexNet & 0.765 & 0.848 & 0.819 & \color{blue}{0.883} & \textbf{0.887} & 0.840 & 0.563 \\
\hline
\end{tabular}
\label{tab:CatsDogsBiased_bias_f1}
\end{table}

\begin{table}[h]
\centering

\caption{CatsDogsBiased. JS divergence}
\begin{tabular}{|l|c|c|c|c|c|c|c|}
\hline
Model & Layer 1 & Layer 2 & Layer 3 & Layer 4 & Layer 5 & Avg. JS  $\downarrow$ & Acc. $\uparrow$ \\ \hline
ResNeXt101 & 0.134 & 0.100 & 0.085 & \color{blue}{0.074} & \textbf{0.069} & 0.092 & 0.914 \\
ResNeXt50 & 0.135 & 0.101 & 0.085 & \color{blue}{0.074} & \textbf{0.069} & 0.093 & 0.876 \\
VGG16 & 0.136 & \textbf{0.062} & \color{blue}{0.073} & 0.097 & 0.089 & 0.091 & 0.784 \\
DenseNet169 & 0.135 & \textbf{0.057} & 0.088 & 0.076 & \color{blue}{0.072} & 0.086 & 0.782 \\
DenseNet121 & 0.135 & \textbf{0.057} & 0.088 & 0.077 & \color{blue}{0.075} & 0.086 & 0.761 \\
Resnet18 & 0.137 & \textbf{0.079} & 0.099 & 0.085 & \color{blue}{0.080} & 0.096 & 0.679 \\
Googlelenet & 0.084 & 0.099 & 0.083 & \textbf{0.075} & \color{blue}{0.082} & 0.084 & 0.643 \\
EfficientNet & 0.099 & 0.111 & \color{blue}{0.082} & 0.097 & \textbf{0.073} & 0.092 & 0.586 \\
AlexNet & 0.132 & 0.084 & 0.101 & \textbf{0.053} & \color{blue}{0.054} & 0.085 & 0.563 \\
\hline
\end{tabular}
\label{tab:CatsDogsBiased_bias_js}
\end{table}

Correlations with Accuracy: F1 (0.175), JS Divergence (0.309)
