# Supplementary material for: Concept-Based Mechanistic Interpretability Using Structured Knowledge Graphs
Source: arXiv:2507.05810 source file (2025-07-08)
Supplement: Supplementary file 2 [file appendix_2.tex]

\appendix
\label{appndx:concepts_sources_prompts}

The following table \ref{tab:concept_prompts} shows the concept categories used for annotation of the dataset with BLIP, along with their respective sources and the prompt templates applied.

\begin{table}[htbp]
\centering

\label{tab:concept-categories-sources-prompts}
\begin{tabular}{|l|l|}
\hline
\textbf{Category} & \textbf{Source/Prompt template} \\
\hline
\textbf{Object Part} & GPT-3.5 generated \\
\cline{2-2}
 & Prompt: ``Does this object visibly have [concept]?'' \\
\hline
\textbf{Color} & GPT-3.5 generated \\
\cline{2-2}
 & Prompt: ``Is there evidence of the color [concept] in this image?'' \\
\hline
\textbf{Scene} & Scene 15 Dataset \cite{scene_concepts_dataset} \\
\cline{2-2}
 & Prompt: ``Is this object in a [concept] setting?'' \\
\hline
\textbf{Material} & Flickr Material Database \cite{materials_concepts_dataset} \\
\cline{2-2}
 & Prompt: ``Is this object made of [concept]?'' \\
\hline
\textbf{Texture} & 15 random samples from from Describable Textures Dataset \cite{textures_concepts_dataset} \\
\cline{2-2}
 & Prompt: ``Does this image contain a [concept] texture?'' \\
\hline
\end{tabular}
\label{tab:concept_prompts}
\caption{Sources of concept categories and their corresponding prompts used to annotate datasets.}

\end{table}
