# Supplementary material for: Concept-Based Mechanistic Interpretability Using Structured Knowledge Graphs
Source: arXiv:2507.05810 source file (2025-07-08)
Supplement: Supplementary file 5 [file moad_cnn.tex]

\label{appndx:moad_cnn}

We report the MOAD CNN metric across five residual layers (L0 to L4) for each model, along with the standard deviation in Table~\ref{tab:moad_dynamic} calculated for the embeddings of Cats/Dogs dataset. Table~\ref{tab:moad_performance} summarizes the overall classification performance of each model.

\begin{table}[ht]
\centering
\caption{MOAD mean and standar values per layer. }
\resizebox{\textwidth}{!}{
\begin{tabular}{lcccccccccc}
\toprule
\textbf{Model} & \multicolumn{2}{c}{L0} & \multicolumn{2}{c}{L1} & \multicolumn{2}{c}{L2} & \multicolumn{2}{c}{L3} & \multicolumn{2}{c}{L4} \\
\cmidrule(lr){2-3} \cmidrule(lr){4-5} \cmidrule(lr){6-7} \cmidrule(lr){8-9} \cmidrule(lr){10-11}
& mean & std & mean & std & mean & std & mean & std & mean & std \\
\midrule
AlexNet     & 0.0115 & 0.0003 & 0.0019 & 0.0003 & 0.0065 & 0.0007 & 0.0106 & 0.0006 & 0.0275 & 0.0027 \\
DenseNet121 & 0.0486 & 0.0002 & 0.0041 & 0.0001 & 0.0032 & 0.0001 & 0.0057 & 0.0001 & 0.0297 & 0.0007 \\
DenseNet169 & {0.0479} & 0.0001 & 0.0036 & 0.0003 & 0.0032 & 0.0001 & 0.0056 & 0.0000 & 0.0186 & 0.0003 \\
EfficientNet& 0.0009 & 0.0001 & 0.0377 & 0.0007 & 0.0130 & 0.0006 & 0.0380 & 0.0013 & {0.0943} & 0.0023 \\
GoogLeNet   & 0.0013 & 0.0000 & 0.0029 & 0.0000 & 0.0088 & 0.0003 & 0.0291 & 0.0012 & {0.1358} & 0.0070 \\
ResNet18    & 0.0041 & 0.0000 & 0.0007 & 0.0000 & 0.0021 & 0.0000 & 0.0062 & 0.0001 & {0.0367} & 0.0010 \\
ResNeXt50   & {0.0616} & 0.0000 & 0.0006 & 0.0000 & 0.0021 & 0.0000 & 0.0029 & 0.0000 & 0.0320 & 0.0003 \\
ResNeXt101  & 0.0609 & 0.0000 & 0.0007 & 0.0000 & 0.0014 & 0.0000 & 0.0024 & 0.0000 & 0.0315 & 0.0003 \\
VGG16       & 0.0078 & 0.0000 & 0.0018 & 0.0001 & {0.0043} & 0.0000 & 0.0039 & 0.0000 & 0.0089 & 0.0001 \\
\bottomrule
\label{tab:moad_dynamic}

\end{tabular}
}
\end{table}

\begin{table}[ht]
\centering
\caption{Mean and standard deviation of performance for each model}
\label{tab:moad_performance}
\begin{tabular}{lcc}
\toprule
{Model} & {Performance (mean)} & {std} \\
\midrule
AlexNet     & 0.5616 & 0.0010 \\
DenseNet121 & 0.7745 & 0.0179 \\
DenseNet169 & 0.8123 & 0.0360 \\
EfficientNet& 0.5777 & 0.0062 \\
GoogLeNet   & 0.6254 & 0.0055 \\
ResNet18    & 0.6303 & 0.0045 \\
ResNeXt50   & 0.8571 & 0.0091 \\
ResNeXt101  & 0.8985 & 0.0020 \\
VGG16       & 0.7920 & 0.0195 \\
\bottomrule
\end{tabular}
\end{table}
