# Supplementary material for: Concept-Based Mechanistic Interpretability Using Structured Knowledge Graphs
Source: arXiv:2507.05810 source file (2025-07-08)
Supplement: Supplementary file 6 [file appendix_1_old.tex]

\appendix
\label{appndx:results}



\subsection{Threshold $\geq$ 0.6}
\begin{table}[htbp]
\centering
\renewcommand{\arraystretch}{1.2}
\begin{tabular}{|l|c|c|c|c|c|c|c|}
\hline
Model & Layer 1 & Layer 2 & Layer 3 & Layer 4 & Layer 5 & Avg & Acc $\uparrow$ \\
\hline
DenseNet121  & 0.100 (0.6) & 0.650 (0.6) & 0.818 (0.6) & \textbf{0.887 (0.6)}  & \textcolor{blue}{0.862 (0.6)} & 0.663 & 0.980 \\
ResNeXt101   & 0.100 (0.6) & 0.643 (0.6) & 0.836 (0.6) & \textcolor{blue}{0.917 (0.6)} & \textbf{0.945 (0.6)}  & 0.688 & 0.980 \\
VGG16        & 0.100 (0.6) & 0.305 (0.6) & 0.530 (0.6) & \textcolor{blue}{0.765 (0.6)} & \textbf{0.807 (0.6)}  & 0.501 & 0.970 \\
DenseNet169  & 0.100 (0.6) & 0.580 (0.6) & 0.776 (0.6) & \textcolor{blue}{0.898 (0.6)} & \textbf{0.939 (0.6)}  & 0.659 & 0.960 \\
EfficientNet-B0 & 0.247 (0.6) & 0.100 (0.6) & 0.362 (0.6) & \textcolor{blue}{0.655 (0.6)} & \textbf{0.958 (0.6)}  & 0.464 & 0.960 \\
GoogLeNet    & 0.247 (0.6) & 0.783 (0.6) & \textcolor{blue}{0.881 (0.6)} & \textbf{0.934 (0.6)} & 0.867 (0.6)         & 0.743 & 0.960 \\
ResNeXt50    & 0.100 (0.6) & 0.670 (0.6) & 0.898 (0.6) & \textbf{0.941 (0.6)} & \textcolor{blue}{0.916 (0.6)}         & 0.705 & 0.960 \\
ResNet18     & 0.100 (0.6) & 0.412 (0.6) & 0.758 (0.6) & \textcolor{blue}{0.789 (0.6)} & \textbf{0.841 (0.6)}  & 0.580 & 0.950 \\
AlexNet      & 0.100 (0.6) & 0.309 (0.6) & 0.705 (0.6) & \textbf{0.801 (0.6)}  & \textcolor{blue}{0.749 (0.6)} & 0.533 & 0.940 \\
\hline
\end{tabular}
\caption{Dataset: HuskyVsWolf (ImageNet)}
\end{table}


\begin{table}[htbp]
\centering
\renewcommand{\arraystretch}{1.2}
\begin{tabular}{|l|c|c|c|c|c|c|c|}
\hline
Model         & Layer 1         & Layer 2         & Layer 3         & Layer 4                   & Layer 5                   & Avg   & Acc $\uparrow$ \\
\hline
ResNeXt101    & 0.276 (0.6)     & 0.654 (0.6)     & 0.851 (0.6)     & \textcolor{blue}{0.941 (0.7)} & \textbf{0.971 (0.7)}      & 0.739 & 0.740 \\
VGG16         & 0.232 (0.6)     & 0.496 (0.9)     & 0.496 (0.9)     & \textcolor{blue}{0.713 (0.6)} & \textbf{0.845 (0.6)}      & 0.557 & 0.710 \\
DenseNet169   & 0.232 (0.6)     & 0.533 (0.6)     & 0.805 (0.6)     & \textbf{0.912 (0.6)}      & \textcolor{blue}{0.907 (0.7)} & 0.678 & 0.700 \\
ResNeXt50     & 0.232 (0.6)     & 0.654 (0.6)     & 0.863 (0.6)     & \textcolor{blue}{0.901 (0.6)} & \textbf{0.916 (0.7)}      & 0.713 & 0.690 \\
DenseNet121   & 0.276 (0.6)     & 0.597 (0.6)     & \textbf{0.875 (0.6)}      & \textcolor{blue}{0.870 (0.6)} & 0.859 (0.6)             & 0.695 & 0.680 \\
ResNet18      & 0.232 (0.6)     & 0.597 (0.6)     & 0.681 (0.6)     & \textcolor{blue}{0.737 (0.6)} & \textbf{0.920 (0.6)}      & 0.634 & 0.670 \\
AlexNet       & 0.262 (0.6)     & 0.552 (0.6)     & \textcolor{blue}{0.700 (0.6)} & 0.672 (0.6)               & \textbf{0.768 (0.6)}      & 0.591 & 0.650 \\
GoogLeNet     & 0.500 (0.6)     & 0.700 (0.6)     & 0.854 (0.6)     & \textbf{0.932 (0.6)}      & \textcolor{blue}{0.914 (0.7)} & 0.780 & 0.620 \\
EfficientNet-B0  & 0.342 (0.6)     & 0.254 (0.6)     & 0.496 (0.9)     & \textcolor{blue}{0.615 (0.6)} & \textbf{0.904 (0.6)}      & 0.523 & 0.600 \\
\hline
\end{tabular}
\caption{Dataset: KitFoxVsRedFox}
\end{table}


\begin{table}[htbp]
\centering
\renewcommand{\arraystretch}{1.2}
\begin{tabular}{|l|c|c|c|c|c|c|c|}
\hline
Model & Layer 1 & Layer 2 & Layer 3 & Layer 4 & Layer 5 & Avg & Acc $\uparrow$ \\
\hline
ResNeXt101    & 0.000 (0.0)     & 0.759 (0.6)     & \textbf{0.934 (0.6)}      & 0.876 (0.6)               & \textcolor{blue}{0.889 (0.6)} & 0.692   & 0.914 \\
ResNeXt50     & 0.000 (0.0)     & 0.725 (0.6)     & \textcolor{blue}{0.906 (0.6)} & 0.876 (0.6)               & \textbf{0.910 (0.6)}      & 0.683   & 0.876 \\
VGG16         & 0.000 (0.0)     & 0.384 (0.6)     & 0.501 (0.6)     & \textcolor{blue}{0.751 (0.6)} & \textbf{0.911 (0.6)}      & 0.509   & 0.784 \\
DenseNet169   & 0.000 (0.0)     & 0.759 (0.6)     & 0.866 (0.6)     & \textcolor{blue}{0.919 (0.6)} & \textbf{0.938 (0.6)}      & 0.697   & 0.782 \\
DenseNet121   & 0.000 (0.0)     & 0.746 (0.6)     & \textbf{0.898 (0.6)}      & 0.876 (0.6)               & \textcolor{blue}{0.896 (0.6)} & 0.683   & 0.761 \\
ResNet18      & 0.000 (0.0)     & 0.447 (0.6)     & 0.772 (0.6)     & \textcolor{blue}{0.819 (0.6)} & \textbf{0.876 (0.6)}      & 0.583   & 0.679 \\
GoogLeNet     & 0.323 (0.6)     & 0.816 (0.6)     & \textcolor{blue}{0.876 (0.6)} & \textbf{0.934 (0.6)}      & 0.841 (0.7)               & 0.758   & 0.643 \\
EfficientNet-B0  & 0.143 (0.6)     & 0.085 (0.6)     & 0.501 (0.6)     & \textcolor{blue}{0.785 (0.6)} & \textbf{0.893 (0.6)}      & 0.481   & 0.586 \\
AlexNet       & 0.000 (0.0)     & 0.386 (0.6)     & \textcolor{blue}{0.731 (0.6)} & \textbf{0.759 (0.6)}      & 0.759 (0.6)               & 0.527   & 0.563 \\
\hline
\end{tabular}
\caption{Dataset: Cats Dogs biased}
\end{table}



\begin{table}[htbp]
\centering
\renewcommand{\arraystretch}{1.2}
\begin{tabular}{|l|c|c|c|c|c|c|c|}
\hline
Model & Layer 1 & Layer 2 & Layer 3 & Layer 4 & Layer 5 & Avg & Acc $\uparrow$ \\
\hline
ResNet18     & 0.159 (0.6)      & 0.357 (0.6)      & 0.495 (0.6)      & \textbf{0.600 (0.6)} & \textcolor{blue}{0.540 (0.6)} & 0.430   & 0.513 \\
DenseNet169  & 0.157 (0.6)      & 0.492 (0.6)      & \textcolor{blue}{0.533 (0.6)} & \textbf{0.550 (0.6)} & 0.469 (0.6)      & 0.440   & 0.492 \\
AlexNet      & 0.357 (0.6)      & 0.465 (0.6)      & 0.469 (0.6)      & \textcolor{blue}{0.558 (0.6)} & \textbf{0.644 (0.6)} & 0.498   & 0.492 \\
GoogLeNet    & 0.230 (0.6)      & \textbf{0.512 (0.6)} & \textcolor{blue}{0.458 (0.6)} & 0.402 (0.6)      & 0.245 (0.6)      & 0.369   & 0.492 \\
VGG16        & 0.134 (0.6)      & 0.258 (0.6)      & 0.479 (0.6)      & \textbf{0.516 (0.6)} & \textcolor{blue}{0.503 (0.6)} & 0.378   & 0.477 \\
EfficientNet-B0 & 0.186 (0.6)      & 0.153 (0.6)      & \textcolor{blue}{0.465 (0.6)} & \textbf{0.528 (0.6)} & 0.378 (0.6)      & 0.342   & 0.472 \\
ResNeXt50    & 0.161 (0.6)      & \textbf{0.553 (0.6)} & \textcolor{blue}{0.434 (0.6)} & 0.384 (0.6)      & 0.331 (0.6)      & 0.372   & 0.447 \\
DenseNet121  & 0.161 (0.6)      & \textbf{0.599 (0.6)} & 0.497 (0.6)      & \textcolor{blue}{0.551 (0.6)} & 0.456 (0.6)     & 0.453   & 0.442 \\
ResNeXt101   & 0.168 (0.6)      & \textcolor{blue}{0.460 (0.6)} & 0.374 (0.6)      & \textbf{0.484 (0.6)} & 0.339 (0.7)      & 0.365   & 0.397 \\
\hline
\end{tabular}
\caption{derm7pt}
\end{table}


\begin{table}[htbp]
\centering
\renewcommand{\arraystretch}{1.2}
\begin{tabular}{|l|c|c|c|c|c|c|c|}
\hline
Model & Layer 1 & Layer 2 & Layer 3 & Layer 4 & Layer 5 & Avg & Acc $\uparrow$ \\
\hline
EfficientNet-B0 & 0.000 (0.0)       & 0.000 (0.0)          & \textcolor{blue}{0.583 (0.6)} & \textbf{1.000 (0.7)}        & \textbf{1.000 (0.6)}         & 0.517 & 0.914 \\
GoogLeNet     & \textcolor{blue}{0.250 (0.6)} & \textbf{1.000 (0.8)} & \textbf{1.000 (0.7)}         & \textbf{1.000 (0.7)}        & \textbf{1.000 (0.6)}         & 0.850 & 0.901 \\
DenseNet169   & \textcolor{blue}{0.000 (0.0)} & \textbf{1.000 (0.8)} & \textbf{1.000 (0.7)}         & \textbf{1.000 (0.7)}        & \textbf{1.000 (0.6)}         & 0.800 & 0.901 \\
DenseNet121   & \textcolor{blue}{0.000 (0.0)} & \textbf{1.000 (0.8)} & \textbf{1.000 (0.7)}         & \textbf{1.000 (0.7)}        & \textbf{1.000 (0.6)}         & 0.800 & 0.888 \\
ResNeXt50     & \textcolor{blue}{0.000 (0.0)} & \textbf{1.000 (0.8)} & \textbf{1.000 (0.7)}         & \textbf{1.000 (0.7)}        & \textbf{1.000 (0.6)}         & 0.800 & 0.868 \\
ResNet18      & 0.000 (0.0)       & \textcolor{blue}{0.500 (0.7)} & \textbf{1.000 (0.8)}         & \textbf{1.000 (0.7)}        & \textbf{1.000 (0.6)}         & 0.700 & 0.865 \\
VGG16         & 0.000 (0.0)       & \textcolor{blue}{0.583 (0.6)} & 0.542 (0.6)                & \textbf{1.000 (0.8)}        & \textbf{1.000 (0.7)}         & 0.625 & 0.851 \\
AlexNet       & 0.000 (0.0)       & \textcolor{blue}{0.583 (0.6)} & \textbf{1.000 (0.8)}         & \textbf{1.000 (0.8)}        & \textbf{1.000 (0.7)}         & 0.717 & 0.848 \\
ResNeXt101    & \textcolor{blue}{0.000 (0.0)} & \textbf{1.000 (0.8)} & \textbf{1.000 (0.8)}         & \textbf{1.000 (0.7)}        & \textbf{1.000 (0.7)}         & 0.800 & 0.812 \\
\hline
\end{tabular}
\caption{Manumoi}
\end{table}

\sofiia{add imagenetpart if we are sure that we are on good direction...}

\newpage
\subsection{Threshold $\geq$ 0.1}

\begin{table}[htbp]
\centering
\renewcommand{\arraystretch}{1.2}
\begin{tabular}{|l|c|c|c|c|c|c|c|}
\hline
Model & Layer 1 & Layer 2 & Layer 3 & Layer 4 & Layer 5 & Avg & Acc $\uparrow$ \\
\hline
DenseNet121  & 0.826 (0.1)     & 0.868 (0.1)     & 0.933 (0.1)     & \textbf{0.973 (0.4)} & \textcolor{blue}{0.970 (0.4)} & 0.914   & 0.980 \\
ResNeXt101   & 0.826 (0.1)     & 0.929 (0.5) & 0.941 (0.4)     & \textbf{0.987 (0.4)} & \textcolor{blue}{0.973 (0.4)} & 0.931   & 0.980 \\
VGG16        & 0.826 (0.1)     & 0.826 (0.1)     & 0.850 (0.1)     & \textcolor{blue}{0.877 (0.4)} & \textbf{0.934 (0.4)} & 0.862   & 0.970 \\
DenseNet169  & 0.826 (0.1)     & 0.872 (0.1)     & 0.923 (0.1)     & \textcolor{blue}{0.969 (0.4)} & \textbf{0.978 (0.4)} & 0.914   & 0.960 \\
EfficientNet-B0 & 0.826 (0.1)     & 0.826 (0.1)     & 0.858 (0.5)     & \textcolor{blue}{0.885 (0.4)} & \textbf{0.958 (0.6)} & 0.871   & 0.960 \\
GoogLeNet    & 0.826 (0.1)     & 0.895 (0.1)     & \textbf{0.957 (0.4)} & \textcolor{blue}{0.949 (0.1)} & 0.940 (0.4)       & 0.913   & 0.960 \\
ResNeXt50    & 0.826 (0.1)     & 0.881 (0.1)     & 0.941 (0.1)     & \textbf{0.984 (0.4)} & \textcolor{blue}{0.978 (0.4)} & 0.922   & 0.960 \\
ResNet18     & 0.826 (0.1)     & 0.885 (0.5)     & 0.875 (0.1)     & \textcolor{blue}{0.926 (0.1)} & \textbf{0.944 (0.1)} & 0.891   & 0.950 \\
AlexNet      & 0.826 (0.1)     & 0.846 (0.5)     & 0.867 (0.1)     & \textbf{0.895 (0.5)} & \textcolor{blue}{0.891 (0.5)} & 0.865   & 0.940 \\
\hline
\end{tabular}
\caption{Dataset: HuskyVsWolf (ImageNet)}
\end{table}


\begin{table}[htbp]
\centering
\renewcommand{\arraystretch}{1.2}
\begin{tabular}{|l|c|c|c|c|c|c|c|}
\toprule
Model         & Layer 1         & Layer 2         & Layer 3         & Layer 4                   & Layer 5                   & Avg   & Acc $\uparrow$ \\
\midrule
ResNeXt101    & 0.831 (0.1)     & 0.925 (0.4)     & 0.941 (0.4)     & \textbf{0.986 (0.3)}      & \textcolor{blue}{0.976 (0.4)} & 0.932 & 0.740 \\
VGG16         & 0.831 (0.1)     & 0.837 (0.1)     & 0.848 (0.5)     & \textcolor{blue}{0.927 (0.4)} & \textbf{0.953 (0.4)}      & 0.879 & 0.710 \\
DenseNet169   & 0.831 (0.1)     & 0.884 (0.4)     & 0.955 (0.4)     & \textbf{0.966 (0.4)}      & \textcolor{blue}{0.964 (0.4)} & 0.920 & 0.700 \\
ResNeXt50     & 0.831 (0.1)     & 0.915 (0.4)     & 0.949 (0.4)     & \textcolor{blue}{0.963 (0.3)} & \textbf{0.985 (0.4)}      & 0.928 & 0.690 \\
DenseNet121   & 0.831 (0.1)     & 0.886 (0.5)     & 0.941 (0.4)     & \textcolor{blue}{0.958 (0.4)} & \textbf{0.985 (0.4)}      & 0.920 & 0.680 \\
ResNet18      & 0.831 (0.1)     & 0.847 (0.1)     & 0.914 (0.4)     & \textcolor{blue}{0.947 (0.4)} & \textbf{0.962 (0.4)}      & 0.900 & 0.670 \\
AlexNet       & 0.831 (0.1)     & 0.847 (0.1)     & 0.909 (0.4)     & \textcolor{blue}{0.910 (0.4)} & \textbf{0.913 (0.4)}      & 0.882 & 0.650 \\
GoogLeNet     & 0.834 (0.1)     & 0.926 (0.4)     & 0.948 (0.4)     & \textcolor{blue}{0.968 (0.4)} & \textbf{0.975 (0.3)}      & 0.930 & 0.620 \\
EfficientNet-B0  & 0.831 (0.1)     & 0.831 (0.1)     & 0.844 (0.1)     & \textcolor{blue}{0.920 (0.4)} & \textbf{0.981 (0.4)}      & 0.881 & 0.600 \\
\bottomrule
\end{tabular}
\caption{Dataset: KitFoxVsRedFox (ImageNet)}
\end{table}


\begin{table}[htbp]
\centering
\renewcommand{\arraystretch}{1.2}
\begin{tabular}{|l|c|c|c|c|c|c|c|}
\hline
Model & Layer 1 & Layer 2 & Layer 3 & Layer 4 & Layer 5 & Avg & Acc $\uparrow$ \\
\hline
ResNeXt101    & 0.879 (0.5)     & 0.895 (0.5)     & \textcolor{blue}{0.934 (0.6)} & \textbf{0.940 (0.5)}      & 0.923 (0.3)               & 0.914   & 0.914 \\
ResNeXt50     & 0.870 (0.5)     & 0.916 (0.5)     & 0.909 (0.5)     & \textbf{0.967 (0.5)}      & \textcolor{blue}{0.930 (0.5)} & 0.918   & 0.876 \\
VGG16         & 0.841 (0.1)     & 0.853 (0.5)     & 0.855 (0.5)     & \textcolor{blue}{0.894 (0.5)} & \textbf{0.930 (0.5)}      & 0.875   & 0.784 \\
DenseNet169   & 0.883 (0.5)     & 0.880 (0.5)     & 0.907 (0.5)     & \textbf{0.947 (0.5)}      & \textcolor{blue}{0.938 (0.6)} & 0.911   & 0.782 \\
DenseNet121   & 0.883 (0.5)     & 0.861 (0.5)     & 0.898 (0.4)     & \textcolor{blue}{0.938 (0.5)} & \textbf{0.963 (0.5)}      & 0.909   & 0.761 \\
ResNet18      & 0.841 (0.1)     & 0.863 (0.5)     & \textcolor{blue}{0.905 (0.5)} & \textbf{0.922 (0.5)}      & 0.895 (0.1)               & 0.885   & 0.679 \\
GoogLeNet     & 0.855 (0.5)     & \textcolor{blue}{0.919 (0.5)} & 0.917 (0.5)     & \textbf{0.934 (0.6)}      & 0.907 (0.5)               & 0.906   & 0.643 \\
EfficientNet-B0  & 0.841 (0.1)     & 0.841 (0.1)     & 0.841 (0.1)     & \textcolor{blue}{0.890 (0.5)} & \textbf{0.916 (0.5)}      & 0.866   & 0.586 \\
AlexNet       & 0.866 (0.5)     & 0.848 (0.5)     & 0.875 (0.5)     & \textcolor{blue}{0.883 (0.5)} & \textbf{0.887 (0.5)}      & 0.872   & 0.563 \\
\hline
\end{tabular}
\caption{Dataset: Cats Dogs biased}
\end{table}


\begin{table}[htbp]
\centering
\renewcommand{\arraystretch}{1.2}
\begin{tabular}{|l|c|c|c|c|c|c|c|}
\hline
Model & Layer 1 & Layer 2 & Layer 3 & Layer 4 & Layer 5 & Avg & Acc $\uparrow$ \\
\hline
ResNet18     & 0.481 (0.1)      & 0.496 (0.5)      & 0.591 (0.5)      & \textbf{0.655 (0.5)} & \textcolor{blue}{0.617 (0.4)} & 0.568   & 0.513 \\
DenseNet169  & 0.482 (0.1)      & 0.576 (0.5)      & \textbf{0.642 (0.5)} & \textcolor{blue}{0.594 (0.4)} & 0.566 (0.4)      & 0.572   & 0.492 \\
AlexNet      & 0.486 (0.1)      & 0.495 (0.1)      & 0.570 (0.5)      & \textcolor{blue}{0.558 (0.6)}      & \textbf{0.644 (0.6)} & 0.550   & 0.492 \\
GoogLeNet    & 0.484 (0.1)      & 0.535 (0.4)      & \textbf{0.645 (0.4)}      & \textcolor{blue}{0.611 (0.4)} & 0.511 (0.1)     & 0.557   & 0.492 \\
VGG16        & 0.480 (0.1)      & 0.485 (0.1)      & 0.493 (0.1)      & \textbf{0.620 (0.5)} & \textcolor{blue}{0.586 (0.4)} & 0.533   & 0.477 \\
EfficientNet-B0 & 0.482 (0.1)      & 0.482 (0.1)      & 0.532 (0.5)      & \textbf{0.576 (0.5)} & 0.525 (0.1)      & 0.519   & 0.472 \\
ResNeXt50    & 0.481 (0.1)      & \textcolor{blue}{0.599 (0.5)} & 0.574 (0.4)      & \textbf{0.604 (0.4)} & 0.569 (0.3)      & 0.565   & 0.447 \\
DenseNet121  & 0.482 (0.1)      & 0.604 (0.5)      & \textbf{0.611 (0.4)}      & \textcolor{blue}{0.609 (0.4)} & 0.568 (0.3)     & 0.575   & 0.442 \\
ResNeXt101   & 0.481 (0.1)      & 0.538 (0.4)      & \textcolor{blue}{0.541 (0.3)} & \textbf{0.555 (0.1)} & 0.508 (0.1)      & 0.525   & 0.397 \\
\hline
\end{tabular}
\caption{derm7pt}
\end{table}



\begin{table}[htbp]
\centering
\renewcommand{\arraystretch}{1.2}
\begin{tabular}{|l|c|c|c|c|c|c|c|}
\hline
Model            & Layer 1                   & Layer 2                   & Layer 3                   & Layer 4                    & Layer 5                    & Avg   & Acc $\uparrow$ \\
\hline
EfficientNet-B0  & \textcolor{blue}{0.833 (0.5)} & 0.721 (0.5)               & 0.804 (0.5)               & \textbf{1.000 (0.7)}         & \textbf{1.000 (0.6)}         & 0.872   & 0.914 \\
GoogLeNet        & \textcolor{blue}{0.833 (0.5)} & \textbf{1.000 (0.8)}         & \textbf{1.000 (0.7)}         & \textbf{1.000 (0.5)}         & \textbf{1.000 (0.6)}         & 0.967   & 0.901 \\
DenseNet169      & \textcolor{blue}{0.700 (0.5)} & \textbf{1.000 (0.8)}         & \textbf{1.000 (0.5)}         & \textbf{1.000 (0.7)}         & \textbf{1.000 (0.5)}         & 0.940   & 0.901 \\
DenseNet121      & \textcolor{blue}{0.521 (0.5)} & \textbf{1.000 (0.8)}         & \textbf{1.000 (0.7)}         & \textbf{1.000 (0.5)}         & \textbf{1.000 (0.6)}         & 0.904   & 0.888 \\
ResNeXt50        & \textcolor{blue}{0.738 (0.5)} & \textbf{1.000 (0.8)}         & \textbf{1.000 (0.7)}         & \textbf{1.000 (0.7)}         & \textbf{1.000 (0.5)}         & 0.948   & 0.868 \\
ResNet18         & 0.521 (0.5)               & \textcolor{blue}{0.798 (0.5)} & \textbf{1.000 (0.8)}         & \textbf{1.000 (0.7)}         & \textbf{1.000 (0.5)}         & 0.864   & 0.865 \\
VGG16            & 0.469 (0.1)               & 0.756 (0.5)               & \textcolor{blue}{0.831 (0.5)} & \textbf{1.000 (0.8)}         & \textbf{1.000 (0.7)}         & 0.811   & 0.851 \\
AlexNet          & 0.533 (0.5)               & \textcolor{blue}{0.798 (0.5)} & \textbf{1.000 (0.8)}         & \textbf{1.000 (0.8)}         & \textbf{1.000 (0.7)}         & 0.866   & 0.848 \\
ResNeXt101       & \textcolor{blue}{0.521 (0.5)} & \textbf{1.000 (0.8)}         & \textbf{1.000 (0.8)}         & \textbf{1.000 (0.5)}         & \textbf{1.000 (0.7)}         & 0.904   & 0.812 \\
\hline
\end{tabular}
\caption{Manumoi}
\end{table}


\subsection{Without finetuning}

The values in the tables correspond to the probability of a concept being detected in the feature map produced by the model at a particular layer (the probability is average (Avg) over all concepts). We identify the threshold that yields the maximum probability and provide its value in parentheses. The rows are sorted in descending order of model's accuracy (Acc $\uparrow$). Cells representing the highest probability for each model are marked in bold, while those with the second-best probability are indicated in blue.

\subsection{Threshold $\geq$ 0.6}
\begin{table}[htbp]
\centering
\renewcommand{\arraystretch}{1.2}
\begin{tabular}{|l|c|c|c|c|c|c|c|}
\hline  
Model & Layer 1 & Layer 2 & Layer 3 & Layer 4 & Layer 5 & Avg & Acc $\uparrow$ \\
\hline  
ResNeXt50 & 0.100 (0.6) & 0.685 (0.6) & 0.898 (0.6) & \textbf{0.925 (0.6)} & \textcolor{blue}{0.912 (0.6)} & 0.704 & 0.750 \\
DenseNet169 & 0.100 (0.6) & 0.580 (0.6) & 0.830 (0.6) & \textcolor{blue}{0.921 (0.6)} & \textbf{0.925 (0.6)} & 0.671 & 0.710 \\
ResNeXt101 & 0.100 (0.6) & 0.677 (0.6) & 0.862 (0.6) & \textbf{0.929 (0.6)} & \textcolor{blue}{0.921 (0.6)} & 0.698 & 0.550 \\
ResNet18 & 0.100 (0.6) & 0.435 (0.6) & 0.724 (0.6) & \textcolor{blue}{0.818 (0.6)} & \textbf{0.824 (0.6)} & 0.580 & 0.500 \\
VGG16 & 0.100 (0.6) & 0.305 (0.6) & 0.530 (0.6) & \textcolor{blue}{0.765 (0.6)} & \textbf{0.807 (0.6)} & 0.501 & 0.480 \\
DenseNet121 & 0.100 (0.6) & 0.628 (0.6) & 0.857 (0.6) & \textcolor{blue}{0.867 (0.6)} & \textbf{0.925 (0.6)} & 0.675 & 0.480 \\
AlexNet & 0.100 (0.6) & 0.309 (0.6) & 0.705 (0.6) & \textcolor{blue}{0.758 (0.6)} & \textbf{0.807 (0.6)} & 0.536 & 0.460 \\
GoogLeNet & 0.247 (0.6) & 0.715 (0.6) & \textbf{0.904 (0.6)} & 0.830 (0.6) & \textcolor{blue}{0.864 (0.6)} & 0.712 & 0.430 \\
InceptionV3 & 0.100 (0.6) & 0.703 (0.6) & 0.824 (0.6) & \textbf{0.928 (0.6)} & \textcolor{blue}{0.898 (0.6)} & 0.691 & 0.390 \\
EfficientNet & 0.247 (0.6) & 0.100 (0.6) & 0.339 (0.6) & \textcolor{blue}{0.674 (0.6)} & \textbf{0.886 (0.6)} & 0.449 & 0.300 \\
\hline  
\end{tabular}
\caption{Dataset: HuskyVsWolf (ImageNet)}
\end{table}

\begin{table}[htbp]
\centering
\renewcommand{\arraystretch}{1.2}
\begin{tabular}{|l|c|c|c|c|c|c|c|}
\hline
Model & Layer 1 & Layer 2 & Layer 3 & Layer 4 & Layer 5 & Average & Accuracy \\
\hline
ResNeXt101 & 0.212 (0.6) & 0.635 (0.6) & 0.842 (0.6) & \textbf{0.919 (0.7)} & \textcolor{blue}{0.874 (0.6)} & 0.696 & 0.560 \\
InceptionV3 & 0.302 (0.6) & 0.778 (0.6) & \textcolor{blue}{0.883 (0.6)} & \textbf{0.957 (0.7)} & \textbf{0.957 (0.7)} & 0.776 & 0.530 \\
ResNeXt50 & 0.212 (0.6) & 0.613 (0.6) & 0.885 (0.6) & \textcolor{blue}{0.907 (0.6)} & \textbf{0.946 (0.7)} & 0.712 & 0.530 \\
VGG16 & 0.212 (0.6) & 0.496 (0.9) & 0.496 (0.9) & \textcolor{blue}{0.704 (0.6)} & \textbf{0.848 (0.6)} & 0.551 & 0.530 \\
AlexNet & 0.302 (0.6) & 0.569 (0.6) & 0.671 (0.6) & \textcolor{blue}{0.726 (0.6)} & \textbf{0.778 (0.6)} & 0.609 & 0.510 \\
GoogLeNet & 0.392 (0.6) & 0.688 (0.6) & 0.784 (0.6) & \textbf{0.941 (0.6)} & \textcolor{blue}{0.890 (0.6)} & 0.739 & 0.510 \\
EfficientNet & 0.257 (0.6) & 0.235 (0.6) & 0.496 (0.9) & \textcolor{blue} {0.749 (0.6)} & \textbf{0.900 (0.7)} & 0.527 & 0.500 \\
DenseNet121 & 0.257 (0.6) & 0.572 (0.6) & 0.856 (0.6) & \textbf{0.902 (0.6)} &  \textcolor{blue}{0.888 (0.6)} & 0.695 & 0.500 \\
ResNet18 & 0.212 (0.6) & 0.572 (0.6) & 0.652 (0.6) & \textcolor{blue}{0.798 (0.6)} & \textbf{0.865 (0.6)} & 0.620 & 0.490 \\
DenseNet169 & 0.212 (0.6) & 0.513 (0.6) & 0.816 (0.6) & \textcolor{blue}{0.909 (0.6)} & \textbf{0.921 (0.7)} & 0.674 & 0.470 \\
\hline
\end{tabular}
\caption{Dataset: KitFoxVsRedFox (ImageNet)}
\end{table}


\begin{table}[htbp]
\centering
\renewcommand{\arraystretch}{1.2}
\begin{tabular}{|l|c|c|c|c|c|c|c|}
\hline
Model & Layer 1 & Layer 2 & Layer 3 & Layer 4 & Layer 5 & Average & Accuracy \\
\hline
EfficientNet & 0.143 (0.6) & 0.085 (0.6) & 0.565 (0.6) & \textbf{0.797} (0.6) & \textcolor{blue}{0.789} (0.6) & 0.476 & 0.664 \\
DenseNet169 & 0.000 (0.0) & 0.759 (0.6) & \textcolor{blue}{0.898} (0.6) & \textbf{0.919} (0.6) & \textbf{0.919} (0.6) & 0.699 & 0.649 \\
InceptionV3 & 0.000 (0.0) & 0.785 (0.6) & 0.836 (0.6) & \textbf{0.877} (0.6) & \textcolor{blue}{0.855} (0.6) & 0.671 & 0.557 \\
AlexNet & 0.000 (0.0) & 0.447 (0.6) & 0.731 (0.6) & \textcolor{blue}{0.759 (0.6)} & \textbf{0.806} (0.6) & 0.548 & 0.548 \\
ResNet18 & 0.000 (0.0) & 0.447 (0.6) & 0.772 (0.6) & \textcolor{blue}{0.866 (0.6)} & \textbf{0.906} (0.6) & 0.598 & 0.538 \\
ResNeXt50 & 0.000 (0.0) & 0.725 (0.6) & \textbf{0.934} (0.6) & \textcolor{blue}{0.932} (0.6) & 0.897 (0.6) & 0.698 & 0.511 \\
VGG16 & 0.000 (0.0) & 0.384 (0.6) & 0.501 (0.6) & \textcolor{blue}{0.751 (0.6)} & \textbf{0.911} (0.6) & 0.509 & 0.511 \\
ResNeXt101 & 0.000 (0.0) & 0.759 (0.6) & 0.887 (0.6) & \textbf{0.910} (0.6) & \textcolor{blue}{0.889} (0.6) & 0.689 & 0.420 \\
DenseNet121 & 0.000 (0.0) & 0.759 (0.6) & \textbf{0.898} (0.6) & \textbf{0.898} (0.6) & \textcolor{blue}{0.896} (0.6) & 0.690 & 0.393 \\
GoogLeNet & 0.323 (0.6) & 0.816 (0.6) & \textcolor{blue}{0.876} (0.6) & \textbf{0.898} (0.6) & 0.836 (0.6) & 0.750 & 0.389 \\
\hline
\end{tabular}
\caption{Dataset: Cats Dogs Cars}
\end{table}


\begin{table}[htbp]
\centering
\renewcommand{\arraystretch}{1.2}
\begin{tabular}{|l|c|c|c|c|c|c|c|}
\hline
Model & Layer 1 & Layer 2 & Layer 3 & Layer 4 & Layer 5 & Average & Accuracy \\
\hline
InceptionV3 & 0.000 (0.0) & \textbf{1.000} (0.8) & \textbf{1.000} (0.8) & \textbf{1.000} (0.7) & \textbf{1.000} (0.6) & 0.800 & 0.297 \\
DenseNet169 & 0.000 (0.0) & \textbf{1.000} (0.8) & \textbf{1.000} (0.7) & \textbf{1.000} (0.7) & \textbf{1.000} (0.7) & 0.800 & 0.287 \\
ResNet18 & 0.000 (0.0) &  \textcolor{blue}{0.500 (0.7)} & \textbf{1.000} (0.8) & \textbf{1.000} (0.7) & \textbf{1.000} (0.8) & 0.700 & 0.267 \\
AlexNet & 0.000 (0.0) &  \textcolor{blue}{0.583 (0.6)} & \textbf{1.000} (0.8) & \textbf{1.000} (0.8) & \textbf{1.000} (0.8) & 0.717 & 0.267 \\
ResNeXt101 & 0.000 (0.0) & \textbf{1.000} (0.8) & \textbf{1.000} (0.7) & \textbf{1.000} (0.7) & \textbf{1.000} (0.7) & 0.800 & 0.241 \\
ResNeXt50 & 0.000 (0.0) & \textbf{1.000} (0.8) & \textbf{1.000} (0.7) & \textbf{1.000} (0.6) & \textbf{1.000} (0.8) & 0.800 & 0.234 \\
VGG16 & 0.000 (0.0) &  \textcolor{blue}{0.583 (0.6)} & 0.542 (0.6) & \textbf{1.000} (0.7) & \textbf{1.000} (0.7) & 0.625 & 0.228 \\
GoogLeNet & 0.250 (0.6) & \textbf{1.000} (0.8) & \textbf{1.000} (0.7) & \textbf{1.000} (0.8) & \textbf{1.000} (0.8) & 0.850 & 0.195 \\
DenseNet121 & 0.000 (0.0) & \textbf{1.000} (0.8) & \textbf{1.000} (0.7) & \textbf{1.000} (0.7) & \textbf{1.000} (0.7) & 0.800 & 0.175 \\
EfficientNet & 0.000 (0.0) & 0.000 (0.0) & \textcolor{blue}{0.750} (0.6) & \textbf{1.000} (0.7) & \textbf{1.000} (0.7) & 0.550 & 0.158 \\
\hline
\end{tabular}
\caption{Dataset: manumoi}
\end{table}

\newpage

\subsection{Threshold $\geq$ 0.1}

\begin{table}[htbp]
\centering
\renewcommand{\arraystretch}{1.2}
\begin{tabular}{|l|c|c|c|c|c|c|c|}
\hline
Model & Layer 1 & Layer 2 & Layer 3 & Layer 4 & Layer 5 & Average & Accuracy \\
\hline
ResNeXt50 & 0.826 (0.1) & 0.888 (0.1) & 0.944 (0.4) & \textcolor{blue}{0.969 (0.4)} & \textbf{0.990 (0.4)} & 0.923 & 0.750 \\
DenseNet169 & 0.826 (0.1) & 0.875 (0.1) & 0.926 (0.1) & \textcolor{blue}{0.978 (0.4)} & \textbf{0.987 (0.4)} & 0.918 & 0.710 \\
ResNeXt101 & 0.826 (0.1) & 0.889 (0.1) & 0.934 (0.1) & \textcolor{blue}{0.975 (0.4)} & \textbf{0.979 (0.4)} & 0.921 & 0.550 \\
ResNet18 & 0.826 (0.1) & 0.872 (0.5) & 0.878 (0.1) & \textbf{0.933 (0.4)} & \textcolor{blue}{0.931 (0.1)} & 0.888 & 0.500 \\
DenseNet121 & 0.826 (0.1) & 0.869 (0.5) & 0.926 (0.1) & \textcolor{blue}{0.968 (0.4)} & \textbf{0.974 (0.4)} & 0.912 & 0.480 \\
VGG16 & 0.826 (0.1) & 0.826 (0.1) & 0.850 (0.1) & \textcolor{blue}{0.877 (0.4)} & \textbf{0.934 (0.4)} & 0.862 & 0.480 \\
AlexNet & 0.826 (0.1) & 0.841 (0.5) & 0.867 (0.1) & \textbf{0.895 (0.5)} &  \textcolor{blue}{0.884 (0.1)} & 0.863 & 0.460 \\
GoogLeNet & 0.826 (0.1) & 0.893 (0.1) & 0.945 (0.4) & \textcolor{blue}{0.955 (0.4)} & \textbf{0.962 (0.4)} & 0.916 & 0.430 \\
InceptionV3 & 0.826 (0.1) & 0.887 (0.1) & 0.962 (0.4) & \textbf{0.997 (0.4)} & \textcolor{blue}{0.973 (0.4)} & 0.929 & 0.390 \\
EfficientNet & 0.826 (0.1) & 0.826 (0.1) &  \textcolor{blue}{0.857 (0.5)} & 0.878 (0.1) & \textbf{0.963 (0.4)} & 0.870 & 0.300 \\
\hline
\end{tabular}
\caption{Dataset: HuskyVsWolf (ImageNet)}
\end{table}

\begin{table}[htbp]
\centering
\renewcommand{\arraystretch}{1.2}
\begin{tabular}{|l|c|c|c|c|c|c|c|}
\hline
Model & Layer 1 & Layer 2 & Layer 3 & Layer 4 & Layer 5 & Avg & Acc $\uparrow$ \\
\hline
ResNeXt101 & 0.825 (0.1) & 0.921 (0.4) & 0.958 (0.4) & \textbf{0.979 (0.4)} & \textcolor{blue}{0.968 (0.4)} & 0.930 & 0.560 \\
InceptionV3 & 0.828 (0.1) & 0.922 (0.4) & \textbf{0.975 (0.4)} & 0.969 (0.4) & \textcolor{blue}{0.971 (0.3)} & 0.933 & 0.530 \\
ResNeXt50 & 0.825 (0.1) & 0.918 (0.4) & 0.962 (0.4) & \textcolor{blue}{0.973 (0.4)} & \textbf{0.975 (0.4)} & 0.931 & 0.530 \\
VGG16 & 0.825 (0.1) & 0.832 (0.1) & 0.850 (0.4) & \textcolor{blue}{0.920 (0.4)} & \textbf{0.954 (0.4)} & 0.876 & 0.530 \\
AlexNet & 0.828 (0.1) & 0.846 (0.5) & 0.904 (0.4) & \textcolor{blue}{0.912 (0.4)} & \textbf{0.917 (0.4)} & 0.882 & 0.510 \\
GoogLeNet & 0.828 (0.1) & 0.929 (0.4) & 0.954 (0.4) & \textbf{0.975 (0.4)} & \textcolor{blue}{0.968 (0.3)} & 0.931 & 0.510 \\
EfficientNet & 0.844 (0.5) & 0.825 (0.1) & 0.838 (0.1) & \textcolor{blue}{0.910 (0.4)} & \textbf{0.971 (0.4)} & 0.878 & 0.500 \\
DenseNet121 & 0.825 (0.1) & 0.885 (0.5) & 0.940 (0.4) & \textcolor{blue}{0.969 (0.4)} & \textbf{0.972 (0.3)} & 0.918 & 0.500 \\
ResNet18 & 0.825 (0.1) & 0.848 (0.1) & 0.909 (0.4) & \textbf{0.954 (0.4)} & \textcolor{blue}{0.949 (0.4)} & 0.897 & 0.490 \\
DenseNet169 & 0.825 (0.1) & 0.881 (0.5) & 0.960 (0.4) & \textcolor{blue}{0.963 (0.3)} & \textbf{0.975 (0.4)} & 0.921 & 0.470 \\
\hline
\end{tabular}
\caption{Dataset: KitFoxVsRedFox (ImageNet)}
\end{table}

\begin{table}[htbp]
\centering
\renewcommand{\arraystretch}{1.2}
\begin{tabular}{|l|c|c|c|c|c|c|c|}
\hline
Model & Layer 1 & Layer 2 & Layer 3 & Layer 4 & Layer 5 & Average & Accuracy \\
\hline
InceptionV3 &  \textcolor{blue}{0.798 (0.5)} &  \textbf{1.000} (0.8) & \textbf{1.000} (0.5) & \textbf{1.000} (0.5) & \textbf{1.000} (0.6) & 0.960 & 0.297 \\
DenseNet169 & 0.688 (0.5) & \textbf{1.000} (0.8) & \textbf{1.000} (0.7) & \textbf{1.000} (0.7) & \textbf{1.000} (0.5) & 0.938 & 0.287 \\
ResNet18 & 0.521 (0.5) & \textcolor{blue}{0.798 (0.5)} & \textbf{1.000} (0.8) & \textbf{1.000} (0.7) & \textbf{1.000} (0.8) & 0.864 & 0.267 \\
AlexNet & 0.750 (0.5) & \textcolor{blue}{0.798 (0.5)} & \textbf{1.000} (0.8) & \textbf{1.000} (0.8) & \textbf{1.000} (0.8) & 0.910 & 0.267 \\
ResNeXt101 & 0.533 (0.5) & \textbf{1.000} (0.8) & \textbf{1.000} (0.7) & \textbf{1.000} (0.5) & \textbf{1.000} (0.7) & 0.907 & 0.241 \\
ResNeXt50 & 0.521 (0.5) & \textbf{1.000} (0.8) & \textbf{1.000} (0.7) & \textbf{1.000} (0.5) & \textbf{1.000} (0.8) & 0.904 & 0.234 \\
VGG16 & 0.469 (0.1) & 0.756 (0.5) & \textcolor{blue}{0.831 (0.5)} & \textbf{1.000} (0.7) & \textbf{1.000} (0.7) & 0.811 & 0.228 \\
GoogLeNet & \textcolor{blue}{0.767 (0.5)} & \textbf{1.000} (0.8) & \textbf{1.000} (0.7) & \textbf{1.000} (0.8) & \textbf{1.000} (0.8) & 0.953 & 0.195 \\
DenseNet121 & \textcolor{blue}{0.688 (0.5)} & \textbf{1.000} (0.8) & \textbf{1.000} (0.7) & \textbf{1.000} (0.7) & \textbf{1.000} (0.5) & 0.938 & 0.175 \\
EfficientNet & \textcolor{blue}{0.833} (0.5) & 0.721 (0.5) & 0.771 (0.5) & \textbf{1.000} (0.7) & \textbf{1.000} (0.7) & 0.865 & 0.158 \\
\hline
\end{tabular}
\caption{Dataset: manumoi}
\end{table}

\begin{table}[htbp]
\centering
\renewcommand{\arraystretch}{1.2}
\begin{tabular}{|l|c|c|c|c|c|c|c|}
\hline
Model & Layer 1 & Layer 2 & Layer 3 & Layer 4 & Layer 5 & Avg & Acc $\uparrow$ \\
\hline
ResNeXt50 & 0.481 (0.1) & 0.575 (0.7) & \textcolor{blue}{0.600 (0.4)} & \textbf{0.627 (0.4}) & 0.532 (0.1) & 0.563 & 0.116 \\

DenseNet169 & 0.482 (0.1) & 0.553 (0.5) & 0.587 (0.4) & \textbf{0.641 (0.4)} & \textcolor{blue}{0.632 (0.7)} & 0.579 & 0.065 \\

ResNeXt101 & 0.481 (0.1) & \textcolor{blue}{0.607 (0.7)} & 0.560 (0.4) & \textbf{0.687 (0.4)} & 0.554 (0.5) & 0.578 & 0.065 \\

DenseNet121 & 0.482 (0.1) & 0.576 (0.6) & \textcolor{blue}{0.662 (0.5)} & \textbf{0.700 (0.7)} & 0.632 (0.9) & 0.610 & 0.065 \\

ResNet18 & 0.481 (0.1) & 0.517 (0.5) & \textcolor{blue}{0.595 (0.7)} & \textbf{0.636 (0.5)} & 0.528 (0.1) & 0.552 & 0.050 \\

InceptionV3 & 0.483 (0.1) & \textbf{0.607 (0.5)} & \textcolor{blue}{0.579 (0.9)} & \textbf{0.607 (0.4)} & 0.526 (0.9) & 0.560 & 0.050 \\

EfficientNet & 0.481 (0.1) & 0.477 (0.1) & \textcolor{blue}{0.530 (0.5) }& \textbf{0.627 (0.5)} & 0.530 (0.6) & 0.529 & 0.050 \\

AlexNet & 0.485 (0.1) & 0.496 (0.1) & \textcolor{blue}{ 0.558 (0.5)} & 0.551 (0.5) & \textbf{0.566 (0.9)} & 0.531 & 0.040 \\

GoogLeNet & 0.487 (0.1) & 0.526 (0.5) & \textcolor{blue}{0.601 (0.4)} & 0.594 (0.5) &\textbf{ 0.611 (0.6)} & 0.564 & 0.040 \\

VGG16 & 0.480 (0.1) & 0.485 (0.1) & 0.493 (0.5) & \textbf{0.572 (0.5)} & \textcolor{blue}{0.534 (0.4)} & 0.513 & 0.035 \\
\hline
\end{tabular}

\caption{Dataset: derm7pt}
\end{table}


\begin{table}[htbp]
\centering
\renewcommand{\arraystretch}{1.2}
\begin{tabular}{|l|c|c|c|c|c|c|c|}
\hline
Model & Layer 1 & Layer 2 & Layer 3 & Layer 4 & Layer 5 & Avg & Acc $\uparrow$ \\
\hline
VGG16 & 0.282 (0.6) & 0.520 (0.6) & \textcolor{blue}{0.695 (0.6)} & \textbf{0.743 (0.6)} & 0.640 (0.6) & 0.576 & 0.737 \\
InceptionV3 & 0.570 (0.6) & \textcolor{blue}{0.693 (0.6)} & \textbf{0.697 (0.6)} & 0.545 (0.6) & 0.582 (0.6) & 0.618 & 0.737 \\
ResNeXt101 & 0.156 (0.6) & \textbf{0.725 (0.6)} & \textcolor{blue}{0.668 (0.6)} & 0.648 (0.6) & 0.477 (0.6) & 0.535 & 0.632 \\
DenseNet121 & 0.238 (0.6) & 0.673 (0.6) & \textbf{0.688 (0.6)} & 0.624 (0.6) & \textcolor{blue}{0.683 (0.6)} & 0.581 & 0.605 \\
DenseNet169 & 0.269 (0.6) & \textbf{0.710 (0.6)} & \textcolor{blue}{0.696 (0.6)} & 0.636 (0.6) & 0.655 (0.6) & 0.593 & 0.579 \\
GoogLeNet & 0.492 (0.6) & \textbf{0.705 (0.6)} & 0.676 (0.6) & \textcolor{blue}{0.640 (0.6)} & 0.571 (0.6) & 0.617 & 0.526 \\
EfficientNet & 0.269 (0.6) & 0.225 (0.6) & \textcolor{blue}{ 0.646 (0.6)} & \textbf{0.730 (0.6)} & 0.628 (0.6) & 0.499 & 0.447 \\
AlexNet & 0.422 (0.6) & \textbf{0.692 (0.6)} & \textcolor{blue}{0.659 (0.6)} & 0.617 (0.6) & 0.625 (0.6) & 0.603 & 0.368 \\
ResNet18 & 0.304 (0.6) & 0.678 (0.6) & \textbf{0.726 (0.6)} & \textcolor{blue}{0.704 (0.6)} & 0.653 (0.6) & 0.613 & 0.368 \\
ResNeXt50 & 0.274 (0.6) &\textbf{ 0.723 (0.6)} & \textcolor{blue}{0.629 (0.6)} & 0.613 (0.6) & 0.457 (0.6) & 0.539 & 0.263 \\
\hline
\end{tabular}

\caption{Dataset: husky wolf with big dataset bias}
\end{table}


\begin{table}[htbp]
\centering
\renewcommand{\arraystretch}{1.2}
\begin{tabular}{|l|c|c|c|c|c|c|c|}
\hline
Model & Layer 1 & Layer 2 & Layer 3 & Layer 4 & Layer 5 & Average & Accuracy \\
\hline
ResNeXt50 & \textbf{0.002} (0.1) & \textbf{0.002} (0.1) & \textbf{0.002} (0.1) & 0.001 (0.1) & 0.001 (0.1) & 0.002 & \textbf{0.938} \\
VGG16 & 0.000 (0.0) & 0.000 (0.0) & 0.000 (0.0) & \textbf{0.002} (0.2) & \textbf{0.002} (0.1) & 0.001 & 0.839 \\
InceptionV3 & \textbf{0.003} (0.5) & 0.002 (0.2) & 0.002 (0.1) & 0.001 (0.1) & 0.001 (0.1) & 0.002 & 0.798 \\
ResNet18 & 0.002 (0.1) & 0.002 (0.3) & 0.002 (0.1) & \textbf{0.003} (0.2) & 0.002 (0.1) & 0.002 & 0.792 \\
AlexNet & 0.002 (0.1) & \textbf{0.002} (0.4) & \textcolor{blue}{0.003} (0.3) & \textcolor{blue}{0.003} (0.3) & 0.002 (0.1) & 0.003 & 0.711 \\
\hline
\end{tabular}
\caption{Dataset: imagenet part = bizarre ! maybe too many concepts + few are relevent for each class (like 4/3000+)}
\end{table}



\begin{table}[htbp]
\centering
\renewcommand{\arraystretch}{1.2}
\begin{tabular}{|l|c|c|c|c|c|c|c|}
\hline
Model & Layer 1 & Layer 2 & Layer 3 & Layer 4 & Layer 5 & Average & Accuracy \\
\hline
EfficientNet & 0.841 (0.1) & 0.841 (0.1) & 0.841 (0.1) & \textcolor{blue}{0.868} (0.5) & \textbf{0.911} (0.1) & 0.861 & 0.664 \\
DenseNet169 & 0.879 (0.5) & 0.880 (0.5) & \textcolor{blue}{0.935} (0.5) & \textbf{0.984} (0.5) & 0.927 (0.3) & 0.921 & 0.649 \\
InceptionV3 & 0.841 (0.1) & 0.871 (0.5) & \textbf{0.932} (0.4) &  \textcolor{blue}{0.929 (0.3)} & 0.907 (0.3) & 0.896 & 0.557 \\
AlexNet & \textbf{0.896} (0.5) & 0.848 (0.5) & 0.875 (0.5) & \textcolor{blue}{0.883 (0.5)} & 0.865 (0.5) & 0.873 & 0.548 \\
ResNet18 & 0.841 (0.1) & 0.874 (0.5) & 0.905 (0.5) & \textbf{0.926} (0.5) & \textcolor{blue}{0.906} (0.6) & 0.891 & 0.538 \\
ResNeXt50 & 0.870 (0.5) & 0.916 (0.5) & 0.934 (0.6) &  \textcolor{blue}{0.948 (0.4)} & \textbf{0.965} (0.5) & 0.926 & 0.511 \\
VGG16 & 0.841 (0.1) & 0.853 (0.5) & 0.855 (0.5) & \textcolor{blue}{ 0.894 (0.5)} & \textbf{0.911} (0.6) & 0.871 & 0.511 \\
ResNeXt101 & 0.879 (0.5) & 0.916 (0.5) & 0.897 (0.5) & \textbf{0.931} (0.3) & \ \textcolor{blue}{0.913} (0.3) & 0.907 & 0.420 \\
DenseNet121 & 0.879 (0.5) & 0.865 (0.5) & 0.898 (0.4) & \textbf{0.974} (0.5) & \textcolor{blue}{0.912} (0.3) & 0.906 & 0.393 \\
GoogLeNet & 0.841 (0.1) & 0.919 (0.5) & \textbf{0.934} (0.5) & \textcolor{blue}{0.927 (0.3)} & \textbf{0.934} (0.3) & 0.911 & 0.389 \\
\hline
\end{tabular}
\caption{Dataset: Cats Dogs Cars}
\end{table}
